# Supplementary material for: Evolution of X-ray and optical rapid variability during the low/hard state in the 2018 outburst of MAXI J1820+070 = ASASSN-18ey
Source: arXiv:2411.03602 ancillary file (2024-11-06)
Supplement: Supplementary file 1 [file si-a18ey-shot-analyses-r1.pdf]

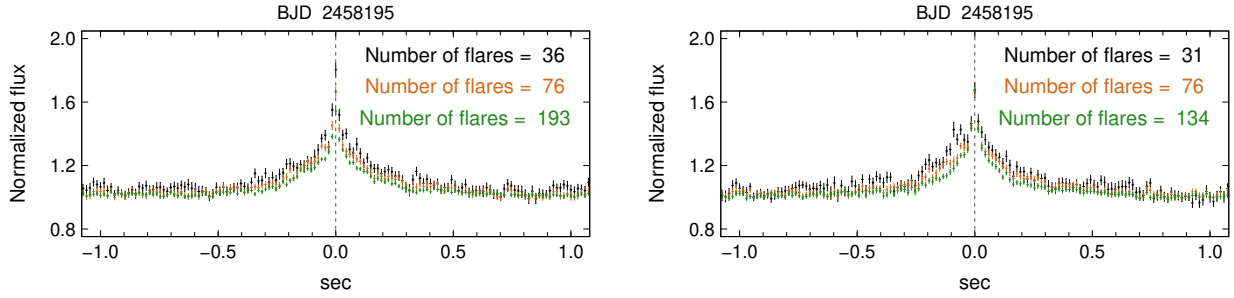

**Fig. E1.** (Left) Comparison of the three optical shot profiles with the three different values of  $t_{\text{int}}$ . The black, orange, and green profiles denote the shot profiles with  $t_{\text{int}} = 10$  s, 5 s, and 2 sec, respectively. The number of flares superposed for one shot profile is given at the right top. (Right) Comparison of the three optical shot profiles with the three different values of  $R_{\text{near}}$ . The black, orange, and green profiles denote the shot profiles with  $R_{\text{near}} = 0.4$ , 0.3, and 0.2, respectively. The number of flares superposed for one shot profile is given at the right top.

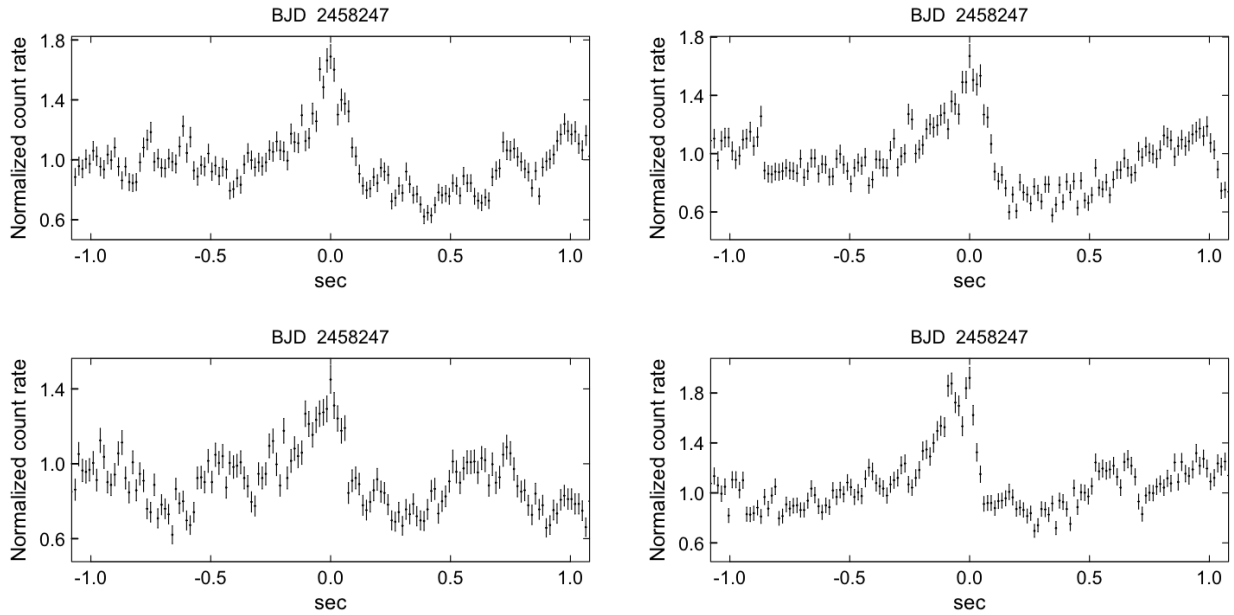

**Fig. E2.** Examples of X-ray flares selected by our shot analysis on BJD 2458247.

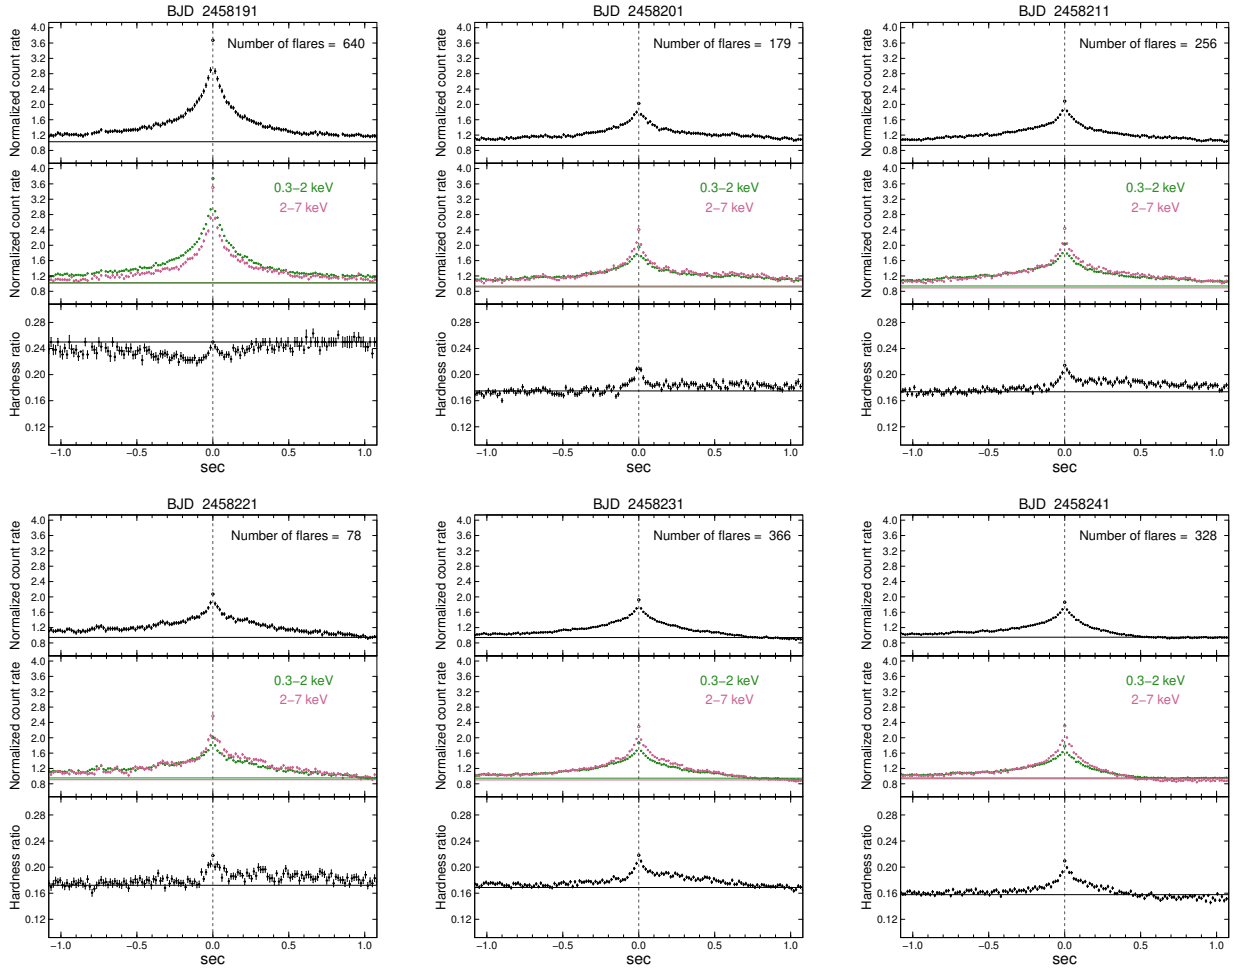

**Fig. E3.** Examples of X-ray shots averaged per date during the 2018 outburst in MAXI J1820+070. We give the number of flares superposed for one shot profile is given in the top panel. The top panel displays the X-ray shot profile in the 0.3–7 keV band (black). The middle panel shows the soft X-ray shot in the 0.3–2 keV band (green) and the hard X-ray shot in the 2–7 keV band (pink). The bottom panel is the 2–7 keV / 0.3–2 keV hardness ratio of the X-ray shot. The horizontal lines in the top and middle panels represent the average flux level outside of flares at  $|t| > 2.5$  s. The horizontal line in the bottom panel represents the average hardness ratio.

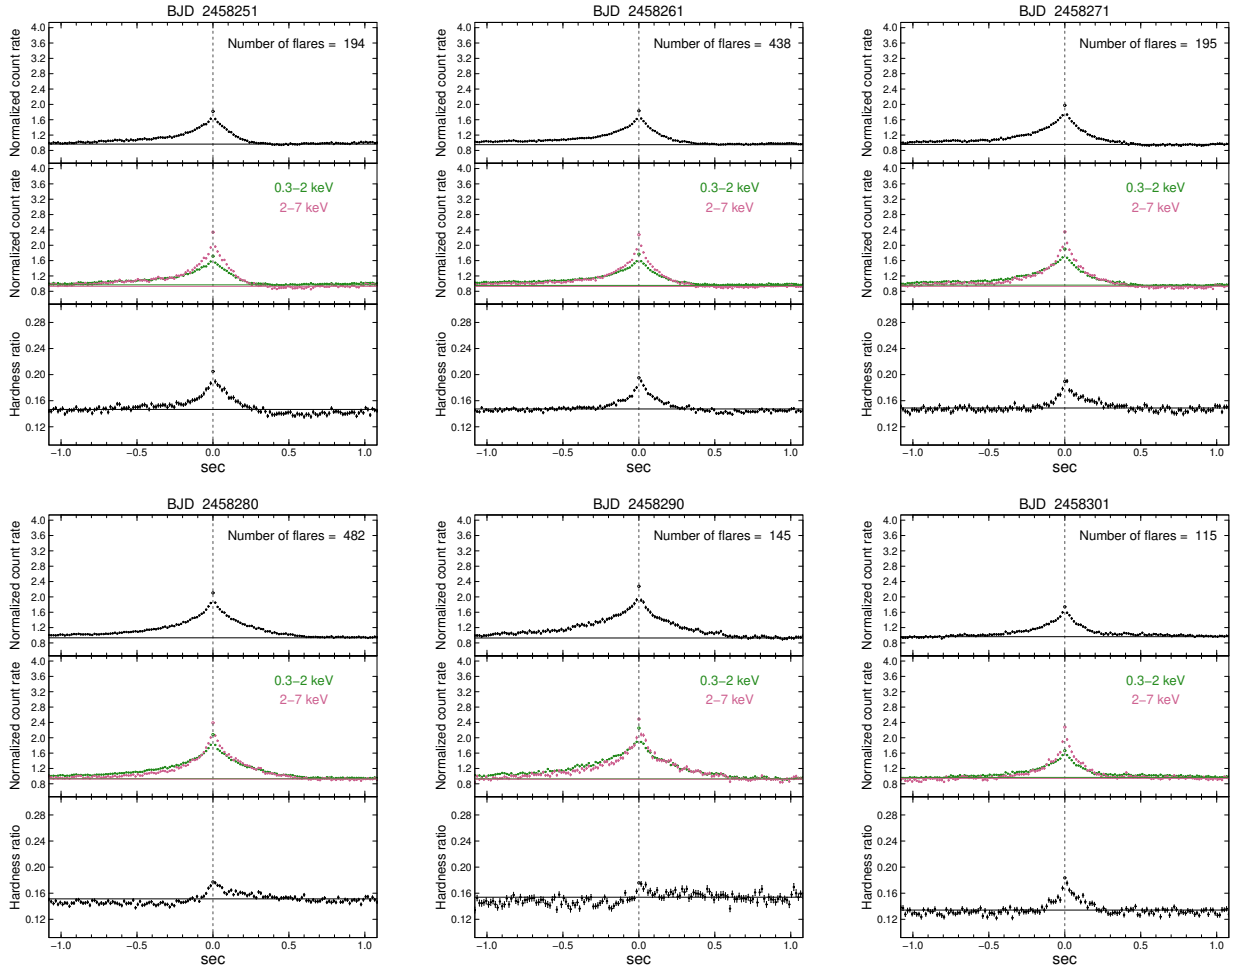

**Fig. E3.** Examples of X-ray shots averaged per date during the 2018 outburst in MAXI J1820+070 (continued). We give the number of flares superposed for one shot profile is given in the top panel. The top panel displays the X-ray shot profile in the 0.3–7 keV band (black). The middle panel shows the soft X-ray shot in the 0.3–2 keV band (green) and the hard X-ray shot in the 2–7 keV band (pink). The bottom panel is the 2–7 keV / 0.3–2 keV hardness ratio of the X-ray shot. The horizontal lines in the top and middle panels represent the average flux level outside of flares at  $|t| > 2.5$  s. The horizontal line in the bottom panel represents the average hardness ratio.

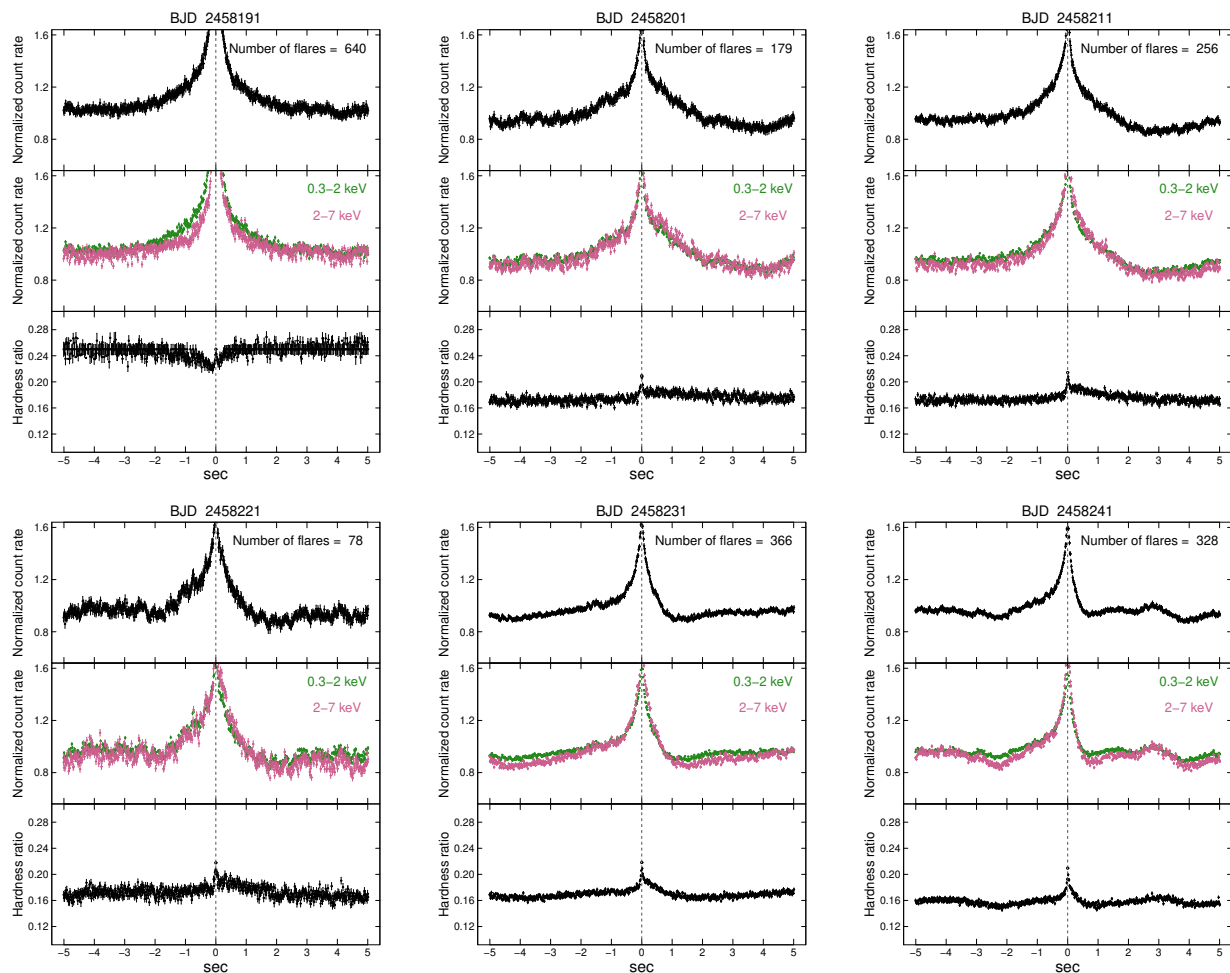

**Fig. E4.** Examples of wide X-ray shots averaged per date during the 2018 outburst in MAXI J1820+070. We give the number of flares superposed for one shot profile is given in the top panel. The top panel displays the X-ray shot profile in the 0.3–7 keV band (black). The middle panel shows the soft X-ray shot in the 0.3–2 keV band (green) and the hard X-ray shot in the 2–7 keV band (pink). The bottom panel is the 2–7 keV / 0.3–2 keV hardness ratio of the X-ray shot.

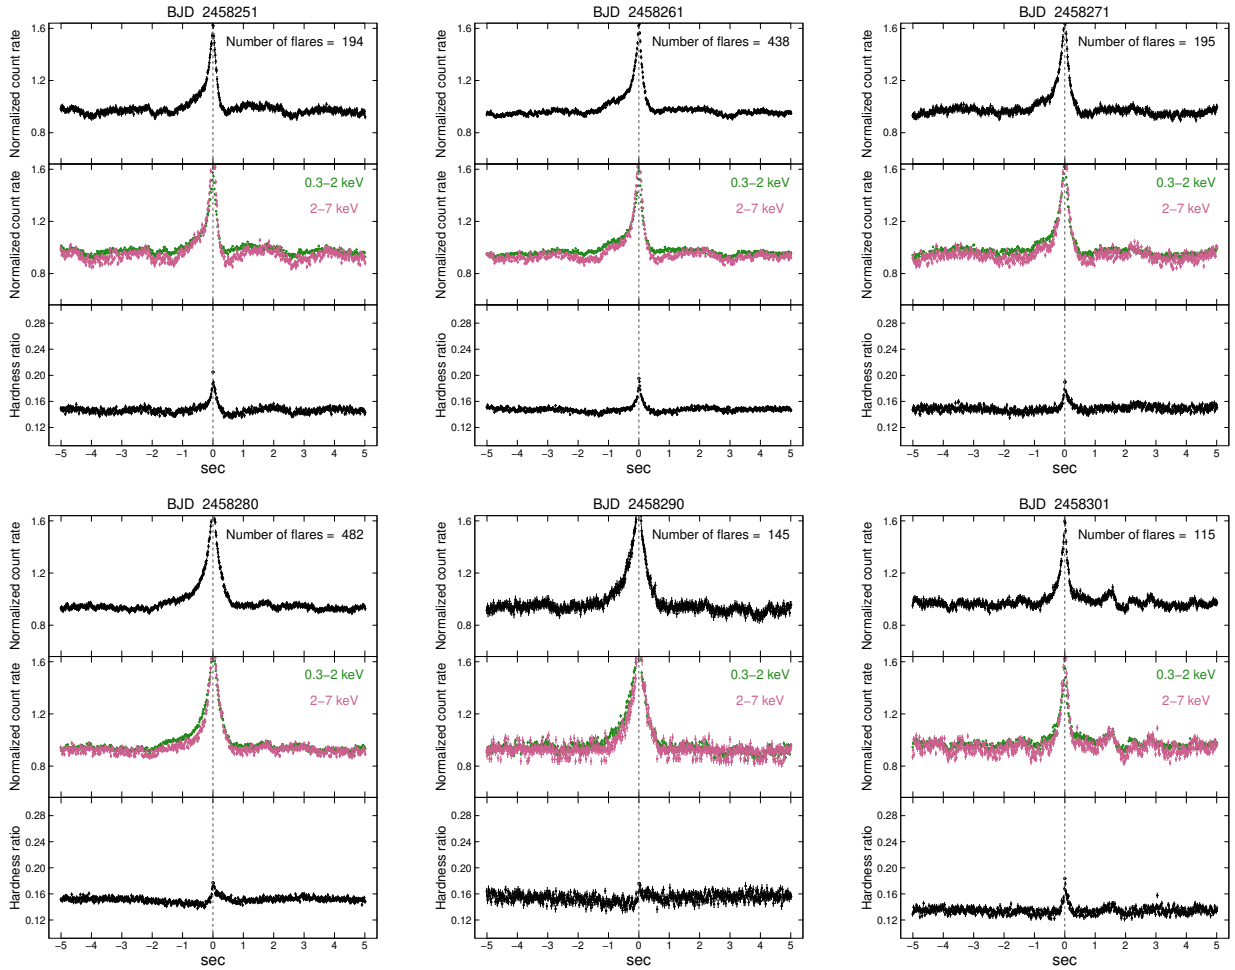

**Fig. E4.** Examples of wide X-ray shots averaged per date during the 2018 outburst in MAXI J1820+070 (continued). We give the number of flares superposed for one shot profile is given in the top panel. The top panel displays the X-ray shot profile in the 0.3–7 keV band (black). The middle panel shows the soft X-ray shot in the 0.3–2 keV band (green) and the hard X-ray shot in the 2–7 keV band (pink). The bottom panel is the 2–7 keV / 0.3–2 keV hardness ratio of the X-ray shot.

**Table E1.** Log of observations of MAXI J1820+070 = ASASSN-18ey with Tomo-e Gozen.

| Start*   | End*     | Mag <sup>†</sup> | Error <sup>‡</sup> | N <sup>§</sup> | Exp <sup>  </sup> |
|----------|----------|------------------|--------------------|----------------|-------------------|
| 192.2800 | 192.2955 | 12.460           | 0.130              | 20000          | 0.0665            |
| 192.2979 | 192.3057 | 12.451           | 0.128              | 10000          | 0.0665            |
| 194.2519 | 194.2523 | 12.193           | 0.221              | 600            | 0.0665            |
| 194.2922 | 194.2936 | 12.333           | 0.272              | 8000           | 0.0147            |
| 194.2951 | 194.3074 | 12.293           | 0.197              | 64000          | 0.0147            |
| 194.3305 | 194.3347 | 12.293           | 0.508              | 24000          | 0.0147            |
| 194.3362 | 194.3376 | 12.288           | 0.393              | 8000           | 0.0147            |
| 194.3390 | 194.3475 | 12.223           | 0.224              | 48000          | 0.0147            |
| 195.2985 | 195.3330 | 11.978           | 0.164              | 184000         | 0.0147            |
| 195.3360 | 195.3388 | 11.955           | 0.164              | 16000          | 0.0147            |
| 200.2622 | 200.2758 | 12.315           | 1.610              | 72000          | 0.0147            |
| 200.3095 | 200.3109 | 11.718           | 0.187              | 8000           | 0.0147            |
| 200.3297 | 200.3311 | 11.709           | 0.163              | 8000           | 0.0147            |
| 218.2783 | 218.2897 | 11.943           | 0.153              | 64000          | 0.0147            |
| 222.3049 | 222.3119 | 11.641           | 0.112              | 40000          | 0.0147            |
| 228.3137 | 228.3222 | 12.060           | 0.182              | 48000          | 0.0147            |
| 230.3000 | 230.3140 | 12.120           | 0.128              | 80000          | 0.0147            |
| 239.2494 | 239.2592 | 12.284           | 0.111              | 56000          | 0.0147            |
| 239.2621 | 239.2700 | 12.300           | 0.119              | 40000          | 0.0147            |
| 239.3008 | 239.3078 | 12.258           | 0.127              | 40000          | 0.0147            |
| 243.2994 | 243.3141 | 12.284           | 0.247              | 80000          | 0.0147            |
| 249.1681 | 249.2113 | 12.434           | 0.108              | 240000         | 0.0147            |

\*BJD – 2458000.0.

<sup>†</sup>Mean magnitude.<sup>‡</sup>1 $\sigma$  of mean magnitude.<sup>§</sup>Number of observations.<sup>||</sup>Exposure time in units of seconds.

**Table E2.** Log of observations of MAXI J1820+070 = ASASSN-18ey with NICER.

| NICER ObsID | Start*   | End*     | On-source time <sup>†</sup> | Average rate <sup>‡</sup> |
|-------------|----------|----------|-----------------------------|---------------------------|
| 1200120101  | 190.0778 | 190.4164 | 7105                        | 819.5                     |
| 1200120102  | 191.1126 | 191.4461 | 5827                        | 1467.7                    |
| 1200120103  | 191.4980 | 192.4757 | 11028                       | 2118.0                    |
| 1200120104  | 192.5277 | 193.3767 | 7376                        | 3247.4                    |
| 1200120105  | 193.6873 | 194.3332 | 3059                        | 5321.7                    |
| 1200120106  | 198.8875 | 199.4695 | 5485                        | 19650.3                   |
| 1200120107  | 199.5262 | 200.4378 | 18311                       | 19099.3                   |
| 1200120108  | 200.4903 | 200.7672 | 6976                        | 16848.2                   |
| 1200120109  | 201.5295 | 202.4394 | 13352                       | 20297.2                   |
| 1200120110  | 202.4845 | 203.4685 | 23048                       | 20186.9                   |
| 1200120111  | 203.5135 | 204.4422 | 18045                       | 19779.3                   |
| 1200120113  | 205.8380 | 206.4782 | 1999                        | 18593.1                   |
| 1200120114  | 206.5400 | 206.9424 | 3206                        | 18419.7                   |
| 1200120115  | 207.8894 | 207.9783 | 3457                        | 18048.7                   |
| 1200120116  | 208.8549 | 209.3158 | 11004                       | 18252.4                   |
| 1200120117  | 209.8204 | 209.9594 | 3212                        | 17799.3                   |
| 1200120118  | 210.5285 | 210.9978 | 10542                       | 17927.2                   |
| 1200120119  | 211.8162 | 211.9597 | 3425                        | 18012.4                   |
| 1200120120  | 212.5245 | 213.0514 | 8069                        | 18105.8                   |
| 1200120121  | 213.8143 | 214.2681 | 3449                        | 18451.4                   |
| 1200120122  | 214.7787 | 215.3671 | 4056                        | 18201.0                   |
| 1200120123  | 215.8093 | 215.9420 | 1237                        | 17890.0                   |
| 1200120124  | 218.2568 | 218.3302 | 727                         | 18020.1                   |
| 1200120125  | 219.2872 | 219.4900 | 1789                        | 18201.5                   |
| 1200120126  | 219.5511 | 220.0011 | 1792                        | 18004.1                   |
| 1200120127  | 220.9048 | 221.4200 | 1712                        | 17650.3                   |
| 1200120129  | 223.5444 | 223.7498 | 796                         | 17889.9                   |
| 1200120130  | 224.5704 | 225.4933 | 10504                       | 17065.4                   |
| 1200120131  | 225.5345 | 226.0733 | 7511                        | 16983.4                   |
| 1200120132  | 228.6312 | 228.7765 | 3827                        | 17771.6                   |
| 1200120133  | 229.5395 | 229.8705 | 4823                        | 17571.9                   |
| 1200120134  | 230.4890 | 230.8360 | 7030                        | 17590.4                   |
| 1200120135  | 231.5347 | 231.8671 | 4344                        | 17828.0                   |
| 1200120136  | 232.9541 | 233.4064 | 1708                        | 17851.7                   |
| 1200120137  | 233.5334 | 234.4408 | 7033                        | 17374.5                   |
| 1200120138  | 234.4938 | 235.3133 | 4219                        | 17335.0                   |
| 1200120139  | 235.8458 | 236.4098 | 879                         | 17307.6                   |
| 1200120140  | 238.0778 | 238.4766 | 2612                        | 17727.9                   |
| 1200120141  | 239.8173 | 239.8279 | 904                         | 17397.9                   |
| 1200120142  | 240.7356 | 240.9376 | 5573                        | 17124.9                   |
| 1200120143  | 241.7487 | 241.9019 | 3970                        | 17068.3                   |
| 1200120144  | 242.7784 | 242.9310 | 5123                        | 17186.7                   |
| 1200120145  | 243.7449 | 243.9560 | 6351                        | 17220.3                   |
| 1200120146  | 244.7790 | 245.0466 | 5464                        | 16995.2                   |
| 1200120147  | 245.7388 | 245.9466 | 5101                        | 17369.5                   |
| 1200120148  | 246.6435 | 246.9719 | 4249                        | 17515.5                   |
| 1200120149  | 247.7336 | 247.9340 | 2650                        | 17778.1                   |
| 1200120150  | 248.6985 | 248.7703 | 1774                        | 17803.0                   |
| 1200120151  | 249.7924 | 249.9256 | 1178                        | 17248.2                   |
| 1200120152  | 250.7574 | 251.4742 | 2704                        | 17329.7                   |
| 1200120153  | 251.7868 | 251.9829 | 1033                        | 17531.4                   |

**Table E2.** Log of observations of MAXI J1820+070 = ASASSN-18ey with NICER (Continued).

| NICER ObsID | Start*   | End*     | On-source time <sup>†</sup> | Average rate <sup>‡</sup> |
|-------------|----------|----------|-----------------------------|---------------------------|
| 1200120154  | 252.7524 | 252.9477 | 733                         | 17518.1                   |
| 1200120155  | 259.5792 | 259.9046 | 1228                        | 16037.1                   |
| 1200120156  | 260.7392 | 260.9526 | 6591                        | 15769.9                   |
| 1200120157  | 261.7073 | 261.9169 | 5224                        | 14536.9                   |
| 1200120158  | 262.7397 | 262.9470 | 2599                        | 13617.7                   |
| 1200120159  | 263.7136 | 263.9110 | 2053                        | 13101.5                   |
| 1200120160  | 264.6796 | 264.9245 | 2509                        | 12509.4                   |
| 1200120161  | 265.5680 | 265.8231 | 4092                        | 12522.9                   |
| 1200120162  | 266.7225 | 266.9253 | 2781                        | 12260.3                   |
| 1200120163  | 267.7523 | 267.9547 | 3327                        | 12873.4                   |
| 1200120164  | 268.7166 | 268.9175 | 2507                        | 12560.4                   |
| 1200120165  | 269.7469 | 269.9495 | 3030                        | 11915.6                   |
| 1200120166  | 270.7131 | 270.9148 | 2663                        | 11658.6                   |
| 1200120167  | 271.7423 | 271.9447 | 2290                        | 11312.8                   |
| 1200120168  | 272.7059 | 272.7783 | 1144                        | 11163.0                   |
| 1200120169  | 273.7625 | 273.9364 | 2105                        | 10077.7                   |
| 1200120170  | 274.7005 | 274.9094 | 4179                        | 10217.3                   |
| 1200120171  | 275.8586 | 275.8860 | 2373                        | 9526.3                    |
| 1200120172  | 276.6971 | 276.7875 | 2454                        | 9461.3                    |
| 1200120173  | 277.7892 | 277.8805 | 3282                        | 8672.7                    |
| 1200120174  | 278.7679 | 278.8443 | 2714                        | 8153.2                    |
| 1200120175  | 279.6788 | 279.7963 | 2254                        | 7721.2                    |
| 1200120176  | 280.6274 | 280.8387 | 5965                        | 7354.2                    |
| 1200120177  | 281.6729 | 281.7415 | 901                         | 7001.7                    |
| 1200120178  | 282.8736 | 282.9533 | 2630                        | 6472.6                    |
| 1200120179  | 283.9037 | 283.9753 | 1255                        | 6254.4                    |
| 1200120180  | 284.7407 | 284.8814 | 2246                        | 5993.5                    |
| 1200120181  | 285.5290 | 285.5337 | 405                         | 5366.9                    |
| 1200120182  | 286.9308 | 286.9527 | 1896                        | 5318.7                    |
| 1200120183  | 288.0388 | 288.0493 | 904                         | 5338.0                    |
| 1200120184  | 289.1348 | 289.1444 | 833                         | 5315.3                    |
| 1200120185  | 289.5834 | 290.1711 | 2570                        | 5291.0                    |
| 1200120186  | 292.6001 | 293.1129 | 1825                        | 6314.0                    |
| 1200120187  | 293.8981 | 293.9715 | 1405                        | 6836.3                    |
| 1200120188  | 296.9097 | 296.9329 | 1964                        | 8842.0                    |
| 1200120189  | 297.6993 | 298.4682 | 16061                       | 9869.2                    |
| 1200120190  | 298.5326 | 299.3148 | 2815                        | 10916.5                   |
| 1200120191  | 300.2592 | 300.2682 | 749                         | 12349.1                   |
| 1200120192  | 301.0301 | 301.0406 | 820                         | 13979.5                   |
| 1200120193  | 301.7996 | 301.8079 | 712                         | 14871.4                   |
| 1200120194  | 302.5718 | 302.7297 | 5268                        | 16214.3                   |
| 1200120195  | 304.3824 | 304.3905 | 691                         | 24291.0                   |
| 1200120196  | 304.7778 | 305.4970 | 6508                        | 28373.6                   |

\*BJD–2458000.0.

<sup>†</sup>Units of seconds.<sup>‡</sup>NICER count rate in 0.3–7 keV in units of counts/sec.
